# Supplementary material for: Do Large Language Models Speak All Languages Equally? A Comparative Study in Low-Resource Settings
Source: arXiv:2408.02237 source file (2024-08-05)
Supplement: Supplementary file 1 [file appendix-a.1.tex]

\section{Data Details}

This section presents the detailed data distributions used in our study.
